# Supplementary material for: CodeScope: An Execution-based Multilingual Multitask Multidimensional Benchmark for Evaluating LLMs on Code Understanding and Generation
Source: arXiv:2311.08588 source file (2024-06-07)
Supplement: Supplementary file 1 [file code_sum_additional_analysis.tex]

\subsection{Additional Analysis}

\subsubsection{Code Summarization}
\label{appendix:code_summ}
We report in Figure 5 the per-language overall performance of models across 43 popular languages. The detailed experimental results are elaborated in Table \ref{table:code_sum_result_lang}. We find that all models have relatively stable performance across languages, indicating that the LLM have gained generic code understanding regardless of the syntax and grammar differences. Among them, it has been observed that languages with higher readability or simpler grammar, such as Python, Ruby, and PHP, tend to yield better performance in the evaluated metrics (provide a citation if available). On the other hand, LLMs show a notable lack of familiarity with assembly languages, resulting in an average drop of 21\% in performance when compared to high-level languages like Python. This discrepancy can be attributed to the fact that most of the training corpus for LLMs primarily consists of high-level languages, while assembly language, with its distinct grammar, is not well-represented. 

To further investigate the dynamics of LLMs' code summarization capability with code length, we evenly divided the test samples into three groups(short, median, and long) based on the distribution of lines of code (LOC). This division was determined by considering the position of each code sample within the overall distribution of LOC in the specific programming language being analyzed. Since metrics leveraging n-gram overlaps may be more sensitive to the noises in shorter code summarization, we use the BERTScore to analyze the performance change in different LOC-group in Table \ref{table:code_summ_LOC}. As depicted in Figure \ref{fig:code_summ_LOC_BERTScore_linechart}, though GPTs and StarCoder maintain a relatively stable summarization performance across different code length, most model showcase a clear drop of performance with the increase of code length.

% \begin{figure}[htbp]
%     \centering
%     \includegraphics[width=0.5\textwidth]{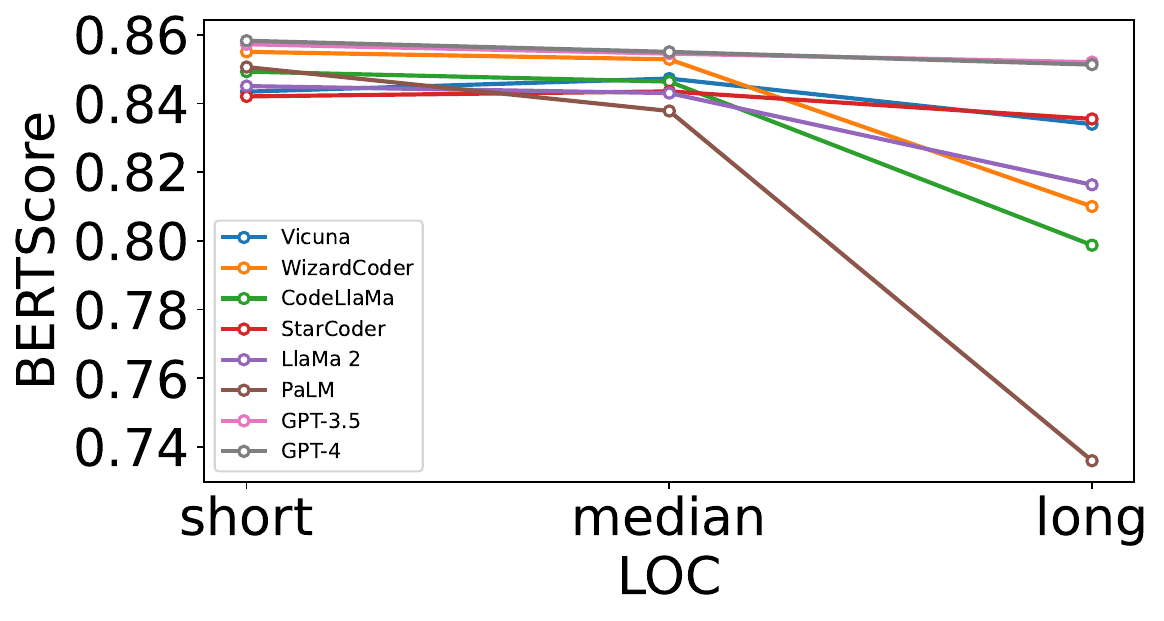}
%     \caption{LLMs' per LOC-level performance on code summarization}
%     \label{fig:code_summ_LOC_BERTScore_linechart}
% \end{figure}

% \begin{figure*}[htbp]
%     \centering
%     \includegraphics[width=\textwidth]{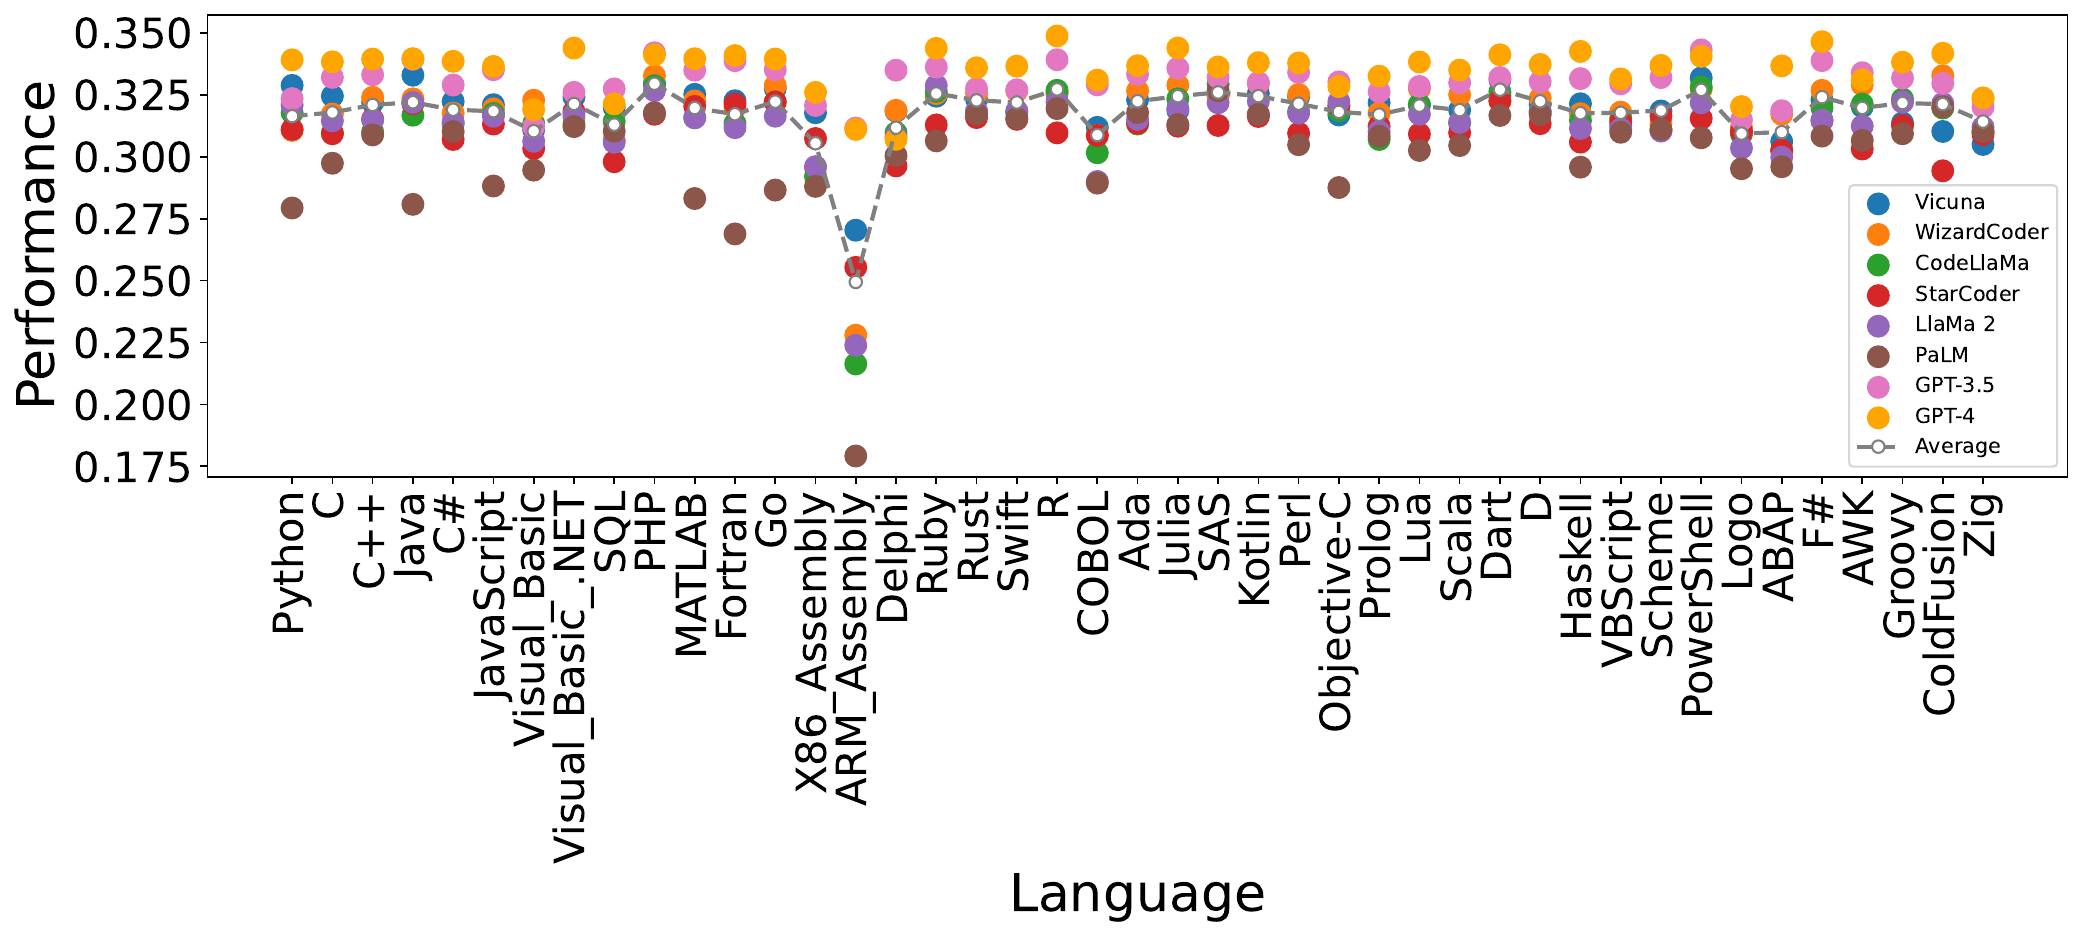}
%     \caption{LLMs' per language performance on code summarization}
%     \label{fig:code_summ_lang_overall_scatterchart}
% \end{figure*}
